# Supplementary material for: An adaptive certified space-time reduced basis method for nonsmooth parabolic partial differential equations
Source: arXiv:2212.13744 source file (2022-12-28)
Supplement: Supplementary file 1 [file 7_Appendix.tex]

\section{Appendix - Problem Fixes}
\label{sec: appendix}
Of course now the question is if we obtain
\begin{align*}
\MBnote{
\Delta_{\calP^\delta}(\mu) = \mathcal{O}(\Delta t)
}
\end{align*}
again and \MBnote{if we can apply the same technique for the RB-DEIM error estimation. I think the answer to the latter is yes, but I will focus on the details after feedback / talk with you.} For the former note that
\begin{align}
\label{eq: projection_appendix}
\|e_\ell(\mu) - \calP^\delta e_\ell(\mu)\| \leq \|y_\delta(\mu) - \calP^\delta y_\delta(\mu) \| + \|y_\ell(\mu) - \calP^\delta y_\ell(\mu) \|.
\end{align}
Thus an argument analogously to the proof of Proposition \ref{prop: time_convergence} using the stability estimates (Lemma \ref{lem: stability_FE} and Lemma \ref{lem: stability_RB}) implies
\begin{align*}
\|e_\ell(\mu) - \calP^\delta e_\ell(\mu)\|_{L^2(I;\Hs)} = \mathcal{O}(\Delta t).
\end{align*}
\MBnote{Note that we either need to modify the proof above or also need to show this estimate w.r.t. the $\test$-norm.}
\newline
Some Remarks:
\begin{enumerate}
\item I tried to avoid the overestimation in \eqref{eq: projection_appendix} and directly show a stability estimate for $e_\ell(\mu)$, which was unfortunately unsuccessful. The way we handle the monotonicity in the proof of Lemma \ref{lem: stability_FE} wasn't transferable.
\item At least for numerical verification of the actual size of the additional estimator term, we could directly use the new $\Delta_{\calP^\delta}$ without the overestimation from \eqref{eq: projection_appendix}. This should also be possible in the old setting given that we can fix it.
\end{enumerate}

%%%%%%%%%%%%%%%%

\subsection{Inf-Sup Constant}
\label{sec: InfSup}
In this section we generalize Proposition 2.9 in \cite{Urb14}. Let us denote 
\begin{align*}
\scrC \colon \Vs \rightarrow \Vs', \quad \scrC \define -\Delta,
\end{align*}
with induced bilinear form $\calC = \langle \scrC \cdot, \cdot \rangle_{\Vs', \Vs}$. Note that
\begin{align}
\label{eq: calB_scrC}
\calB(\phi, \varphi; \mu) = \langle \dot{\phi} + c(\mu) \scrC \phi, \varphi \rangle_{\test', \test} = \langle \scrC^{-1} \dot{\phi} + c(\mu) \phi, \varphi\rangle_{\test}
\end{align} 
for $\phi \in \trial$, $\varphi \in \test$. Which is a consequence of $\langle \scrC \phi, \varphi \rangle_{\test', \test} = \langle \phi, \varphi\rangle_{\test}$, because $\langle \scrC \phi(t), \varphi(t)\rangle_{\Vs',\Vs} = \langle \phi(t), \varphi(t) \rangle_{\Vs}$ for all $t \in I$. The invertibility of $\scrC$ follows e.g. due to its uniform monotonicity by the Browder-Minty theorem (cf., e.g. \cite[Theorem 10.49]{Ren04}). We start with an estimate for the inf-sup constant in the continuous setting.

\begin{proposition}
\label{prop: inf_sup_cont}
For $\beta^\mathrm{LM}(\mu)=\min\{1, c(\mu)\}$ we have all $\mu \in \mathscr P$: 
\begin{align}
\label{eq: inf_sup_cont}
\beta^\mathrm{LM}(\mu) \leq \inf\limits_{\phi \in \trial} \sup\limits_{\varphi \in \test} \frac{\calB(\phi, \varphi; \mu)}{\|\phi\|}_{\trial, \delta} \|\varphi\|_{\test}\quad\text{for all }\pmu\in\mathscr P.
\end{align}
Moreover, if $c(\mu) = 1$ for all $\mu \in \mathscr P$, then equality holds in \eqref{eq: inf_sup_cont}.
\end{proposition}
\begin{proof}
Let $\mu \in \mathscr P$ be arbitrary but fixed. For $\phi \in \trial$ we estimate
\begin{align*}
\|\scrC^{-1} \dot{\phi} + c(\mu) \phi \|_{\test}^2 & = \|\scrC^{-1} \dot{\phi} \|_{\test}^2 + c^2(\mu) \|\phi\|_{\test}^2 + 2 c(\mu) \langle \scrC^{-1} \dot{\phi}, \phi \rangle_{\test}\\
& = \|\dot{\phi}\|_{L^2(I;\Vs')}^2 + c^2(\mu) \|\phi\|_{\test}^2 + c(\mu) \|\phi(T)\|_{\Hs}^2\\
& \geq \min\{1, c(\mu), c^2(\mu)\} \|\phi\|_\trial^2,
\end{align*}
since $\phi(0) = 0$, which implies 
\begin{align}
\label{eq: inf_sup_cont_proof}
\|\scrC^{-1} \dot{\phi} + c(\mu) \phi \|_{\test} \geq \min\{1, c(\mu)\} \|\phi\|_{\trial},
\end{align}
because $\min\{1, c(\mu), c^2(\mu)\} = \min\{1, c^2(\mu)\}$.
Since for every $z \in \test$ there exists a unique $\psi \in \trial$ such that
\begin{align*}
 \calB(\psi, \varphi; \mu) = \langle z, \varphi\rangle_{\test} \quad \text{for all } \varphi \in \test
\end{align*}
holds, we obtain $z = \scrC^{-1} \dot{\psi} + c(\mu) \psi$, by \eqref{eq: calB_scrC}.
Now for arbitrary $\phi \in \trial$ we can conclude from \eqref{eq: calB_scrC} and \eqref{eq: inf_sup_cont_proof} that
\begin{align*}
\sup\limits_{z \in \test} \frac{\calB(\phi, z; \mu)}{\|z\|_{\test}} & = \sup\limits_{\psi \in \trial} \frac{\calB(\phi, \scrC^{-1} \dot{\psi} + c(\mu) \psi; \mu)}{\|\scrC^{-1} \dot{\psi} + c(\mu) \psi\|_{\test}}\\
& = \sup\limits_{\psi \in \trial} \frac{\langle \scrC^{-1} \dot{\phi} + c(\mu) \phi, \scrC^{-1} \dot{\psi} + c(\mu) \psi \rangle_{\test}}{\|\scrC^{-1} \dot{\psi} + c(\mu) \psi\|_{\test}}\\
& = \|\scrC^{-1}\dot{\phi} + c(\mu) \phi \|_{\test}\\\geq \min\{1, c(\mu)\} \|\phi\|_{\trial},
\end{align*}
where equality in the second to last line follows by choosing $\psi = \phi$ for one direction and using the Cauchy-Schwarz inequality for the other.
\newline 
If $c(\mu) = 1$ independently of $\mu$, then it is easy to see from the first lines of the proof, that we can sharpen \eqref{eq: inf_sup_cont_proof} and obtain
\begin{align*}
\|\scrC^{-1} \dot{\phi} + c(\mu) \phi \|_{\test}^2 = \|\phi\|_\trial^2.
\end{align*}
The second statement readily follows.
\end{proof}

Next we turn to the discrete setting. For $\phi \in \trial$ we set 
\begin{align}
\label{eq: trial_averaged}
\bar{\phi}^k = \frac{1}{\Delta t_k} \int\limits_{I_k} \phi\, \mathrm{d}t \in \Vs, \quad \bar{\phi} = \sum\limits_{k = 1}^K \mathbbm{1}_{I_k} \otimes \bar{\phi}^k \in L^2(I; \Vs). 
\end{align}
Utilizing \eqref{eq: trial_averaged} we define the $(\trial, \delta)$-norm as
\begin{align*}
{\|\phi\|}_{\trial, \delta}^2 \define{\|\bar{\phi}\|}_\test^2 + {\|\dot{\phi}\|}_{\mathscr Y'}^2 + {\|\phi(T)\|}_\Hs^2\quad\text{for }\phi\in \trial_\delta.
\end{align*}
Recall that $\dot{\phi} \in L^2(I;\Hs)$ for $\phi \in \trial_\delta$.

\begin{lemma}
\label{lem: W0T_property_disc}
We have
\begin{align*}
{\langle \dot{\phi}, \bar\phi\rangle}_{L^2(I;H)} = \frac{1}{2} {\|\phi(T)\|}_\Hs^2\quad\text{for all }\phi\in\trial_\delta.
\end{align*}
\end{lemma}
\begin{proof}
Let $\phi\in\trial_\delta$ be chosen arbitrarily. The claim follows from $\calP^\delta\phi=\bar\phi$ and 
\begin{align*}
{\langle \dot{\phi}, \bar{\phi} \rangle}_{L^2(I;\Hs} &= \sum\limits_{k = 1}^K \int\limits_{I_k} {\langle \dot{\phi}(t), \bar{\phi}(t) \rangle}_{\Hs}\, \mathrm{d} t\\
& = \sum_{k = 1}^K \int_{I_k} \frac{1}{2 \Delta t_k}{\langle \phi(t_k) - \phi(t_{k-1}), \phi(t_k) + \phi(t_{k-1})\rangle}_{\Hs} \,\mathrm{d} t\\
& = \frac{1}{2} \sum_{k = 1}^K {\|\phi(t_k)\|}_\Hs^2 - {\|\phi(t_{k-1})\|}_\Hs^2 = \frac{1}{2} {\|\phi(T)\|}_\Hs^2,
\end{align*}
where we have used that $\phi(0) = 0$.
\end{proof}

Now we can proceed analogously to the proof of Proposition~\ref{prop: inf_sup_cont}. 

\begin{proposition}
\label{prop: inf_sup_disc}
For $\beta^\mathrm{LB}=\min\{1, c(\mu)\}$ we have
\begin{align}
\label{eq: inf_sup_disc}
\min\{1, c(\mu)\} \leq \inf\limits_{\phi\in\trial_\delta}\sup\limits_{\varphi\in\test_\delta} \frac{\calB(\phi, \varphi; \mu)}{\|\phi\|_{\trial, \delta} \|\varphi\|_{\test}}\quad\text{for all }\mu\in\mathscr P.
\end{align}
Furthermore if $c(\mu) = 1$ for all $\mu \in \mathscr P$, then equality holds in \eqref{eq: inf_sup_disc}.
\end{proposition}

\begin{proof}
Let $\mu \in \mathscr P$ be arbitrary but fixed. For $\phi \in \trial_\delta$ denote $\bar{\phi}$ as defined in \eqref{eq: trial_averaged}. We can estimate
\begin{align*}
\|\scrC^{-1} \dot{\phi} + c(\mu) \bar{\phi} \|_{\test}^2 & = \|\scrC^{-1} \dot{\phi} \|_{\test}^2 + c^2(\mu) \|\bar{\phi}\|_{\test}^2 + 2 c(\mu) \langle \scrC^{-1} \dot{\phi}, \bar{\phi}\rangle_{\test}\\
& = \|\dot{\phi}\|_{L^2(I;\Vs')}^2 + c^2(\mu) \|\bar{\phi}\|_{\test}^2 + c(\mu) \|\phi(T)\|_\Hs^2\\
& \geq \min\{1, c(\mu), c^2(\mu)\} \|\phi\|_{\trial, \delta}^2,
\end{align*}
since $\langle \scrC^{-1} \dot{\phi}, \bar{\phi} \rangle_\test = \langle \dot{\phi}, \bar{\phi} \rangle_{\test', \test} = \frac{1}{2} \|\phi(T)\|_\Hs^2$ by Lemma \ref{lem: W0T_property_disc}. This implies
\begin{align}
\label{eq: inf_sup_disc_proof1}
\|\scrC^{-1} \dot{\phi} + c(\mu) \bar{\phi} \|_{\test} \geq \min\{1, c(\mu)\} \|\phi\|_{\trial, \delta}.
\end{align}
Assume that for every $z \in \test_\delta$ there exists a unique $\psi \in \trial_\delta$ such that
\begin{align}
\label{eq: inf_sup_disc_proof2}
\langle z, \varphi \rangle_{\test} = \calB(\psi, \varphi; \mu) \quad \text{for all } \varphi \in \test_\delta
\end{align}
holds. We will prove this later. Since $\varphi \in \test_\delta$ is piecewise constant in time, \eqref{eq: calB_scrC} implies that
\begin{align}
\label{eq: inf_sup_disc_proof3}
\calB(\psi, \varphi; \mu)  = \langle \scrC^{-1} \dot{\psi} + c(\mu) \bar{\psi}, \varphi \rangle_{\test}.
\end{align}
This implies together with \eqref{eq: inf_sup_disc_proof2} that $z = \scrC^{-1} \dot{\psi} + c(\mu) \bar{\psi}$.
Analogously to the proof of Proposition \ref{prop: inf_sup_cont} we can now use \eqref{eq: inf_sup_disc_proof1} to conclude that
\begin{align*}
\sup\limits_{z \in \test_\delta} \frac{\calB(\phi, z; \mu)}{\|z\|_{\test}} \geq \min\{1, c(\mu)\} \|\phi\|_{\trial, \delta} \quad \text{for all } \phi \in \trial_\delta.
\end{align*}
Now it remains to prove \eqref{eq: inf_sup_disc_proof2}: For $i = 1,\ldots, N_h$ let $\eta_i > 0, e_j \in \FEspace$ denote the eigenvalues and $\Hs$-normalized eigenvectors of $\scrC$ restricted to $\FEspace$, i.e. the solutions to
\begin{align}
\label{eq: inf_sup_disc_proof4}
\langle e_i, \zeta \rangle_{\Vs} = \eta_i \langle e_i, \zeta\rangle_{\Hs} \quad \text{for all } \zeta \in \FEspace.
\end{align}
This gives the representation $z = \sum\limits_{k = 1}^K z^k \tau_k \in \test_\delta$ with $z^k = \sum\limits_{i = 1}^{N_h} \zfec_i^k e_i \in \FEspace$. 
\newline
Given $z \in \test_\delta$ we determine $\xi_i^k$ for $k = 1, \ldots, K$ and $i = 1, \ldots, N_h$ as the unique solution to the difference equations
\begin{align}
\label{eq: inf_sup_disc_proof5}
\xi_i^0 = 0, \quad \frac{1}{\Delta t_k} \left(\xi_i^k - \xi_i^{k-1}\right) + \frac{\eta_i}{2} c(\mu) \left(\xi_i^k + \xi_i^{k-1}\right) = \eta_i \zfec_i^k
\end{align}
Next, we define $\psi = \sum\limits_{k = 1}^K\sum\limits_{i = 1}^{N_h} \xi_i^k e_i \sigma_k \in \trial_\delta$. Since $\psi$ is piecewise linear in time, we obtain
\begin{align*}
\bar{\psi} = \sum\limits_{k = 1}^K \mathbbm{1}_{I_k} \otimes \bar{\psi}^k = \sum\limits_{k = 1}^K \frac{\Delta t_k}{2} \left(\psi^k + \psi^{k-1}\right) \tau_k,
\end{align*}
with $\psi^k = \psi(t_k)$.
For arbitrary $\varphi \in \test_\delta$ we can conclude that
\begin{align*}
\langle z, \varphi \rangle_{\test} & = \sum\limits_{k,l = 1}^K \langle z^k, \varphi^k\rangle_{\Vs} \int\limits_0^T \tau_k(t) \tau_l(t) \mathrm{d}t 
= \sum\limits_{k = 1}^K \Delta t_k \langle z^k, \varphi^k\rangle_\Vs\\
& = \sum\limits_{k = 1}^K\sum\limits_{i = 1}^{N_h} \Delta t_k \zfec_i^k \langle e_i, \varphi^k \rangle_{\Vs} 
\overset{\eqref{eq: inf_sup_disc_proof4}}{=} \sum\limits_{k = 1}^K\sum\limits_{i = 1}^{N_h} \Delta t_k \zfec_i^k \eta_i \langle e_i, \varphi^k\rangle_\Hs\\
& \overset{\eqref{eq: inf_sup_disc_proof5}}{=} \sum\limits_{k = 1}^K\sum\limits_{i = 1}^{N_h} \Delta t_k \langle e_i, \varphi^k \rangle_\Hs \Big[\frac{1}{\Delta t_k} \left(\xi_i^k - \xi_i^{k-1}\right) + \frac{\eta_i}{2} c(\mu) \left(\xi_i^k + \xi_i^{k-1}\right)\Big]\\
& = \sum\limits_{k = 1}^K \Big\langle\underbrace{\sum\limits_{i = 1}^{N_h} (\xi_i^k - \xi_i^{k-1}) e_i}_{=\;\psi^k - \psi^{k-1}}, \varphi^k \Big\rangle_\Hs + c(\mu) \sum\limits_{k = 1}^K \frac{\Delta t_k }{2} \Big\langle \underbrace{\sum\limits_{i = 1}^{N_h} (\xi_i^k + \xi_i^{k-1}) e_i}_{=\;\psi^k + \psi^{k-1}}, \varphi^k \Big\rangle_\Vs\\
& = \langle \dot{\psi}, \varphi \rangle + \langle \bar{\psi}, \varphi \rangle_{\test} = \langle \scrC^{-1} \dot{\psi} + c(\mu) \bar{\psi}, \varphi\rangle_{\test} \overset{\eqref{eq: inf_sup_disc_proof3}}{=} \calB(\psi, \varphi; \mu).
\end{align*}
This shows the existence. For the uniqueness assume that $\phi, \psi \in \trial_\delta$ are two solutions of \eqref{eq: inf_sup_disc_proof2}. Then
\begin{align*}
\calB(\phi - \psi, \scrC^{-1} (\dot{\phi} - \dot{\psi}) + c(\mu) (\bar{\phi} - \bar{\psi}); \mu) = 0
\end{align*}
and \eqref{eq: inf_sup_disc_proof3} and \eqref{eq: inf_sup_disc_proof1} imply $\|\phi - \psi\|_{\trial, \delta} = 0$, since $c(\mu) > 0$.
\newline 
If $c(\mu) = 1$ independently of $\mu$, then as in the continuous case we can sharpen \eqref{eq: inf_sup_disc_proof1} and obtain
\begin{align*}
\|\scrC^{-1} \dot{\phi} + c(\mu) \bar{\phi} \|_{\test}^2 = \|\phi\|_{\trial, \delta}^2.
\end{align*}
The second statement readily follows.
\end{proof}
\begin{remark}
It is easy to see that the lower bounds in Propositions~{\em\ref{prop: inf_sup_cont}} and {\em\ref{prop: inf_sup_disc}} can be made independent of $\mu$, due to the Lipschitz continuity of $c$ and the compactness of $\mathscr P$.
\end{remark}
